# Supplementary material for: Losses resistant verification of quantum non-Gaussian photon statistics
Source: arXiv:2408.11590 ancillary file (2024-08-21)
Supplement: Supplementary file 1 [file Supplemental_Material.pdf]

# Losses resistant verification of quantum non-Gaussian photon statistics

Riccardo Checchinato,[1] Jan-Heinrich Littmann,[1] Lukáš Lachman,[2] Jaewon Lee,[1] Sven Höfling,[3] Christian Schneider,[4] Radim Filip,[2] and Ana Predojević[1,*]

[1]*Department of Physics, Stockholm University, 10691 Stockholm, Sweden*
[2]*Department of Optics, Palacký University, 17. listopadu 12, 77146 Olomouc, Czech Republic*
[3]*Technische Physik, Physikalisches Institut and Würzburg-Dresden Cluster of Excellence ct.qmat, Universität Würzburg, Am Hubland, D-97074 Würzburg, Germany*
[4]*Institut of Physics, University of Oldenburg, D-26129 Oldenburg, Germany*

Quantum non-Gaussian states of light have fundamental properties that are essential for a multitude of applications in quantum technology. However, many of these features are difficult to detect using standard criteria due to optical losses and detector inefficiency. As the statistics of light are unknown, the loss correction on the data is unreliable, despite the fact that the losses can be precisely measured. To address this issue, we employ a loss-mitigated verification technique utilising quantum non-Gaussian witnesses, which incorporate the known optical losses and detector inefficiency into their derivation. This approach allows us to address the considerable challenge of experimentally demonstrating unheralded quantum non-Gaussian states of single photons and photon pairs.

## CRITERION FOR SINGLE-PHOTON STATES

Here we derive a quantum non-Gaussianity criterion tailored to a scheme where a beamsplitter (BS) leads a photonic state towards two lossy detectors $D_1$ and $D_2$. In order to model the detector losses a virtual beamsplitter is introduced, which attenuates the measured state before it reaches an ideal detector with unit efficiency. In this context we define the parameter $\eta$ as the transmission of the virtual beamsplitter. The objective is to identify those instances in which a given detector responds to an arbitrary mixture of Gaussian states, given a specific value of the transmission coefficient $\eta$. A pure Gaussian state is $|\xi,\alpha\rangle$ is always a result of applying the displacement $D(\alpha)\equiv\exp\left(\alpha a^\dagger-\alpha^* a\right)$ and the squeezing operator $S(\xi)\equiv\exp\left[\xi\left(a^\dagger\right)^2-\xi^* a^2\right]$ on the vacuum, i.e. $|\xi,\alpha\rangle=D(\alpha)S(\xi)|0\rangle$. For the state $|\xi,\alpha\rangle$, we introduce the probability $P_{1,\eta}(\xi,\alpha)$ of a click on $D_1$ and the probability $P_{2,\eta}(\xi,\alpha)$ of simultaneous click on both $D_1$ and $D_2$. In order to identify analytical expressions for these probabilities, we introduce a lossy channel with transmission coefficient $T$ and define $P_0(T,\xi,\alpha)$ as a probability of the vacuum state leaving the lossy channel when the state $|\xi,\alpha\rangle$ enters it. The probability $P_0(T,\xi,\alpha)$ works out to be [1]

$$P_0(T,\xi,\alpha)=\frac{2}{\mu(\xi,T)\mu(-\xi,T)}e^{-\frac{T}{2}\left[\frac{(\alpha+\alpha^*)^2}{4\mu(\xi,T)}-\frac{(\alpha-\alpha^*)^2}{4\mu(-\xi,T)}\right]},\tag{1}$$

where $\mu(\xi,T)\equiv 2e^{\xi}+T\left(1-e^{\xi}\right)$. Eq. (1) allows us to analytically express the probabilities $P_{1,\eta}(\xi,\alpha)$ and $P_{2,\eta}(\xi,\alpha)$ following as:

$$\begin{aligned}P_{1,\eta}(\xi,\alpha)&=1-P_0(\eta/2,\xi,\alpha)\\P_{2,\eta}(\xi,\alpha)&=1-2P_0(\eta/2,\xi,\alpha)+P_0(\eta,\xi,\alpha).\end{aligned}\tag{2}$$

For any given $\eta$, we certify the quantum non-Gaussianity based on measuring the probabilities $P_{1,\eta}$ and $P_{2,\eta}$ by the model detectors. To establish a criterion, we introduce the linear combination

$$F_{\eta,\lambda}(\alpha,\xi)\equiv P_{1,\eta}(\xi,\alpha)+\lambda P_{2,\eta}(\xi,\alpha),\tag{3}$$

where $\lambda$ is a free parameter, and calculate the maximum $F_{\eta,\lambda}=\max_{\xi,\alpha,\phi}F_{\eta,\lambda}(\alpha,\xi,\phi)$ numerically. Consequently, a criterion requires the measured probabilities $P_{1,\eta}$ and $P_{2,\eta}$ satisfy

$$P_{1,\eta}+\lambda P_{2,\eta}>F_{\eta,\lambda}\tag{4}$$

for at least one $\lambda$. We employ numerical approach used in [2] to exclude $\lambda$ from (4), which allows us to derive this criterion only in terms of the probability $P_{1,\eta}$ and $P_{2,\eta}$. In a limit of very small probability $P_{2,\eta}$, we employ Taylor series of formulas in Eq. (2) with respect to $\xi$ and $\alpha$ and consider only the leading members [2]. This allows us to gain an approximate relation between $\alpha$ and $\xi$ maximizing (3) and derive the approximate threshold

$$P_{1,\eta}^3\approx\frac{\eta}{4(2-\eta)}P_{2,\eta},\tag{5}$$

which holds only in the limit $P_{2,\eta}\ll 1$.

## CRITERION FOR COINCIDENCES

We detail the derivation of a criterion for photon coincidences manifested by photon pairs. We consider a general case where the photon pairs occupy $2N$ modes labelled by indices $a_i$ and $b_i$ with $i\in\{1,...,N\}$. Furthermore, we assume a measurement scheme where light in all modes $a_i$ ($b_i$) propagates through a BS and reaches two non-ideal detectors $D_{1,a}$ and $D_{2,a}$ ($D_{1,b}$ and $D_{2,b}$). Such a detection allows us to define the success probability $P_{s,\eta}$ as a coincidence on detectors $D_{1,a}$ and $D_{1,b}$ and the error probability $P_{e,m,\eta}$ as a coincidence on detectors $D_{1,m}$ and $D_{2,m}$ with $m\in\{a,b\}$. Here we discuss

a criterion based on the success probability $P_{s,\eta}$ and the average error probability $P_{e,\eta} \equiv (P_{e,a,\eta} + P_{e,b,\eta})/2$. We aim to reject a set of $2N$-mode Gaussian states $\rho_{\mathcal{G},N}$ of the form

$$\begin{aligned} \rho_{\mathcal{G},N} &= \Pi_{i=1}^{N} \otimes \rho_{i,\xi_i} \\ \rho_{i,\xi_i} &= \frac{1}{1+\xi_i^2} \sum_{n=0}^{\infty} \xi_i^n |n\rangle_{a_i}\langle n| \otimes |n\rangle_{b_i}\langle n|, \end{aligned} \quad (6)$$

where the subscripts $a_i$ ($b_i$) denote the index of the modes measured by the detectors $D_{1,a}$ and $D_{2,a}$ ($D_{1,b}$ and $D_{2,b}$). In the considered scheme, the state $\rho_{\mathcal{G},N}$ yields

$$\begin{aligned} P_{s,\eta}(\boldsymbol{\xi}_N) &= 1 - 2\Pi_{i=0}^{N} \left( \frac{2}{2+\eta\xi_i} \right) \\ &+ \Pi_{i=0}^{N} \left( \frac{4}{4+\xi_i\eta(4-\eta)} \right) \\ P_{e,\eta}(\boldsymbol{\xi}_N) &= 1 - 2\Pi_{i=0}^{N} \left( \frac{2}{2+\eta\xi_i} \right) \\ &+ \Pi_{i=0}^{N} \left( \frac{1}{1+\xi_i\eta} \right), \end{aligned} \quad (7)$$

where $\boldsymbol{\xi}_N = (\xi_1, ..., \xi_N)$ denotes the vector of parameters identifying the state $\rho_{\mathcal{G},N}$. To determine a criterion, we need to maximize the linear combination $F_{\lambda,N}(\boldsymbol{\xi}_N) \equiv P_{s,\eta}(\boldsymbol{\xi}_N) + \lambda P_{e,\eta}(\boldsymbol{\xi}_N)$ over all $\boldsymbol{\xi}_N$ with a fixed $N$. The maximum $F_{\lambda,N} \equiv \max_{\boldsymbol{\xi}} F_{\lambda,N}(\boldsymbol{\xi}_N)$ occurs at $\boldsymbol{\xi}_N$ that fulfills the equation $\nabla F_{\lambda,N}(\boldsymbol{\xi}_N) = 0$. Since solving this equation is difficult for large $N$, we focus only on the limit where $\xi_i \ll 1$ for each $i$, leading to a criterion valid for experimentally relevant states with $P_{e,\eta} \ll 1$. Following the approach in [2, 3], the criterion takes the form $P_{s,\eta} > \max_{\boldsymbol{\xi}_N} T_N(\boldsymbol{\xi}_N)\eta\sqrt{P_{e,\eta}}$, where $T_N(\boldsymbol{\xi}_N)$ reads as:

$$T_N(\boldsymbol{\xi}_N) = \frac{N\bar{\xi}}{\sqrt{N\overline{\xi^2} + N^2\bar{\xi}^2}} \quad (8)$$

with $\bar{\xi} = \sum_{i=1}^{N} \xi_i/N$ and $\overline{\xi^2} = \sum_{i=1}^{N} \xi_i^2/N$. To obtain an explicit form of the criterion, we maximize analytically $T_N(\boldsymbol{\xi}_N)$ over all vectors $\boldsymbol{\xi}_N$. From $\nabla T_N(\boldsymbol{\xi}_N) = 0$ we deduce that the maximum occurs at $\boldsymbol{\xi}_{N,0}$ with identical elements, i.e. $\boldsymbol{\xi}_{N,0} = (\xi_1, ..., \xi_N)$ such that $\xi_i = \xi$ for all $i$ [3]. Inserting $\boldsymbol{\xi}_{N,0}$ into (8) implies the criterion

$$P_{s,\eta} > \eta \frac{N}{2\sqrt{N(N+1)}} \sqrt{P_{e,\eta}}, \quad (9)$$

which imposes a condition parameterized by $\eta$ on the measured probabilities $P_{s,\eta}$ and $P_{e,\eta}$.

We associate depth to a state $\rho$ as the losses $1 - T$ that keep the condition of the criterion in Eq. (8) when evaluating the quantum non-Gaussian coincidences of the state $\rho$ affected by the losses [4]. From Eq. (8), we have

$$T = \frac{2\sqrt{N(N+1)}P_{s,\eta}}{\eta\sqrt{P_{e,\eta}}N}, \quad (10)$$

where $P_{s,\eta}$ and $P_{e,\eta}$ are taken for the state $\rho$ before it enters the lossy channel.

* Electronic address: ana.predojevic@fysik.su.se

[1] M. Fiurášek, L. Lachman and R. Filip. New J. Phys. **23**, 073005 (2021).
[2] I. Straka, et al, npj Quantum Information **4**, 4 (2018)
[3] L. Lachman and R. Filip. Phys. Rev. Lett. **126**, 213604 (2021).
[4] Ivo Straka, et al, Phys. Rev. Lett. **113**, 223603 (2014)
